# Supplementary material for: Universal proximity effect in target search kinetics in the few-encounter limit
Source: arXiv:1611.07788 source file (2016-11-23)
Supplement: Supplementary file 1 [file SI_PRX.pdf]

**Supplementary Information**  
**Universal proximity effect in target search kinetics**

Aljaž Godec<sup>1,2</sup> and Ralf Metzler<sup>1</sup>

<sup>1</sup>*Institute of Physics & Astronomy, University of Potsdam, D-14476 Potsdam-Golm, Germany*

<sup>2</sup>*Department of Molecular Modeling, National Institute of Chemistry, 1000 Ljubljana, Slovenia*

In this Supplementary Information we summarize the calculations leading to the results presented in the main text.

## S1. ON THE LAPLACE TRANSFORM OF THE FPT DENSITY WITH FINITE MOMENTS

In the main text we demand that  $0 < \langle T^n(x_0) \rangle < \infty$  for  $\forall n$ . In other words,  $\tilde{\varphi}(s)$  is the Laplace transform of a normalized smooth density with positive support and is differentiable at zero infinitely many times and therefore admits a power series representation,  $\tilde{\varphi}(s) = \sum_{n=0}^{\infty} (-s)^n \langle T^n(x_0) \rangle / n!$  with a convergence radius  $-\infty < s < \lambda_0$ . We assume that  $\tilde{\varphi}(s)$  has no branch point (at least) in this region of convergence. Moreover, we limit the discussion to the situations, in which  $\lim_{n \rightarrow \infty} \frac{g^{(n)}}{h^{(n)}} < \infty$  (in fact it turns out that  $\lim_{n \rightarrow \infty} \frac{g^{(n)}}{h^{(n)}} = 0$ ). Both assumptions are satisfied in all systems/models addressed herein. Herefrom follows the representation [1]

$$\tilde{\varphi}(s) = \frac{g(s; x_0)}{h(s; x_a)} = \frac{\sum_{k=0}^{\infty} g^{(k)}(x_0) s^k / k!}{\sum_{k=0}^{\infty} h^{(k)}(x_a) s^k / k!} = \sum_{n=0}^{\infty} \frac{(-s)^n}{n!} \langle T^n \rangle, \quad (\text{S1})$$

where

$$\langle T^n \rangle = (-1)^n \frac{g^{(n)}}{h^{(0)}} - \sum_{k=1}^n (-1)^k \binom{n}{k} \frac{h^{(k)}}{h^{(0)}} \langle T^{n-k} \rangle. \quad (\text{S2})$$

All  $g^{(n)}, h^{(n)}$  must be finite and the moment expansion in Eq. (S1) converges for  $-\infty < \text{Re}(s) < \lambda_0$ . The positivity and finiteness of the moments impose bounds on  $g^{(n)}, h^{(n)}$ , which are, however, not sharp [2]. It appears, nevertheless, that these bounds generally assure  $\lim_{n \rightarrow \infty} \frac{g^{(n)}}{h^{(n)}} < \infty$  (see specific examples in S3). Moreover, the roots of the analytic functions  $g(s; x_0)$  and  $h(s; x_a)$  are distinct [1] and the smallest eigenvalue  $-\lambda_0 < 0$  (note that  $\lambda_0$  is real) must be a simple pole of  $\tilde{\varphi}(s)$  as the opposite would imply that the leading order term for  $t \rightarrow \infty$  would be  $\propto t e^{-\lambda_i t}$ . We also demand that  $\tilde{\varphi}(s)$  has no branch points along the negative real axis, which is the case in all studied examples.

## S2. ASYMPTOTIC INVERSION OF $\tilde{\varphi}(s)$

In order to invert  $\tilde{\varphi}(s)$  to obtain the long-time asymptotic we proceed in two steps: a) determining  $\lambda_0$  and b) determining the residue of  $\tilde{\varphi}(s)$  at  $-\lambda_0$ .

a) The first part is rooted in the idea of using the standard Newton iteration [3] for finding roots of non-linear equations. We show here how one can transform it into an exact analytical method. For the present case, where  $-\lambda_0$  is the solution of the equation  $h(s) = \sum_{k=0}^{\infty} h^{(k)}(x_0) s^k / k! = 0$ , which is closest to the origin, this can be uniquely done.

Let the inverse of the function  $h(s) = z : \mathbb{C} \rightarrow \mathbb{C}$  be  $h^{-1}(z) = s$  (which can be multivalued in general) and let  $h(s_0) = 0$  and  $h'(s_0) \neq 0$ , with  $s_r$  being a simple complex root closest to the origin. Moreover, we assume that 0 is a regular point of  $h(s)$  (this is warranted by the assumptions of the preceding section). Expanding  $h^{-1}(z)$  in a Taylor series in the vicinity of 0 we obtain

$$s_r = \frac{\partial h^{-1}(0)}{\partial z} [z(s_r) - z(0)] + \frac{1}{2!} \frac{\partial^2 h^{-1}(0)}{\partial z^2} [z(s_r) - z(0)]^2 + \frac{1}{3!} \frac{\partial^3 h^{-1}(0)}{\partial z^3} [z(s_r) - z(0)]^3 + \dots \quad (\text{S3})$$

Notice that by definition  $z(s_r) = 0$  and  $z(0) = h(0)$  and  $\frac{\partial h^{-1}(0)}{\partial z} \equiv \left( \frac{\partial z}{\partial h^{-1}(0)} \right)^{-1}$  and moreover also  $\frac{\partial z}{\partial h^{-1}(0)} = \frac{\partial h}{\partial s} |_{s=0} \equiv h^{(1)}(0)$ . Therefore, the first order approximation to  $s_r$  is

$$s_1 \approx -\frac{h(0)}{h^{(1)}(0)}. \quad (\text{S4})$$

Plugging this back into Eq. (S3) we have for the second order approximation

$$s_2 = -\frac{h(0)}{h^{(1)}(0)} + \frac{\partial h^{-1}(0)}{\partial z} [z(s_r) - z(s_1)] + \dots \quad (\text{S5})$$

Using as before  $z(s_r) = 0$  and expanding  $z(s_1) = h(s_1)$  around 0 in powers of  $\frac{h(0)}{h^{(1)}(0)}$  we find

$$z(s_1) \equiv h\left(-\frac{h(0)}{h^{(1)}(0)}\right) = h(0) - h^{(1)}(0) \frac{h(0)}{h^{(1)}(0)} + \frac{h^{(2)}(0)}{2!} \left(\frac{h(0)}{h^{(1)}(0)}\right)^2 \dots \quad (\text{S6})$$

Omitting terms of order higher than 2, plugging Eq. (S6) into Eq. (S5) and proceeding as before we obtain the second-order approximation to  $s_r$

$$s_2 \approx s_1 - \frac{h(0)^2}{2!} \frac{h^{(2)}(0)}{[h^{(1)}(0)]^3} \quad (\text{S7})$$

Going over to the third order approximation

$$s_3 = -\frac{h(0)}{h^{(1)}(0)} - \frac{h(0)^2}{2!} \frac{h^{(2)}(0)}{[h^{(1)}(0)]^3} + \frac{\partial h^{-1}(0)}{\partial z} [z(s_r) - z(s_2)] + \dots, \quad (\text{S8})$$

expanding as before in Eq. (S6) and repeating the steps with disregard to orders higher than 3 in Eqs. (S8) and (S6), we obtain the third-order approximation to  $s_r$

$$s_3 \approx s_2 - \frac{h(0)^3}{3!} \left( 3 \frac{[h^{(2)}(0)]^2}{[h^{(1)}(0)]^5} - \frac{h^{(3)}(0)}{[h^{(1)}(0)]^4} \right) \quad (\text{S9})$$

The same steps can be repeated further, giving e.g. for the fourth-order approximation

$$s_4 \approx s_3 - \frac{h(0)^4}{4!} \left( 15 \frac{[h^{(2)}(0)]^3}{[h^{(1)}(0)]^7} - \frac{h^{(2)}(0)h^{(3)}(0)}{[h^{(1)}(0)]^6} + 10 \frac{h^{(4)}(0)}{[h^{(1)}(0)]^5} \right) \quad (\text{S10})$$

and so forth. Up to here we were essentially only step-wise improving the approximations in an iterative fashion exactly as in the Newton's iteration. However, continuing in this manner to fifth order and higher we find, by closer inspection, that apart from the prefactors  $\frac{h(0)^n}{(n-1)!h^{(1)}(0)^{2n-1}}$ , Eqs. (S7)-(S10) are a result of a  $(n-1) \times (n-1)$  almost triangular determinant of the form

$$\det \mathcal{A}_n = \begin{vmatrix} \frac{h^{(2)}}{2!} & \frac{2h^{(3)}}{3!} & \frac{3h^{(4)}}{4!} & \dots & \frac{(n-1)h^{(n)}}{n!} & \frac{nh^{(n+1)}}{(n+1)!} \\ \frac{h^{(1)}}{1!} & \frac{(n+2)h^{(2)}}{2!} & \frac{(2n+3)h^{(3)}}{3!} & \dots & \frac{[(n+1)(n-2)+1]h^{(n-1)}}{(n-1)!} & \frac{[(n+1)(n-1)+1]h^{(n)}}{n!} \\ 0 & \frac{2h^{(1)}}{1!} & \frac{(n+3)h^{(2)}}{2!} & \dots & \frac{[(n+1)(n-3)+2]h^{(n-2)}}{(n-2)!} & \frac{[(n+1)(n-2)+2]h^{(n-1)}}{(n-1)!} \\ 0 & 0 & \frac{3h^{(1)}}{1!} & \dots & \frac{[(n+1)(n-4)+3]h^{(n-3)}}{(n-3)!} & \frac{[(n+1)(n-3)+2]h^{(n-2)}}{(n-2)!} \\ \vdots & \vdots & \ddots & \vdots & \vdots & \vdots \\ \vdots & \vdots & \vdots & \frac{(n-2)h^{(1)}}{1!} & \frac{[2(n+1)-3]h^{(2)}}{2!} & \frac{[3(n+1)-3]h^{(3)}}{3!} \\ 0 & 0 & \dots & 0 & \frac{(n-1)h^{(1)}}{1!} & \frac{2nh^{(2)}}{2!} \end{vmatrix}. \quad (\text{S11})$$

Explicitly, the  $i, j$  element of the square matrix  $\mathcal{A}_n$  is

$$\mathcal{A}_n(i, j) = \frac{h^{(i-j+2)}\theta(i-j+1)}{(i-j+2)!} (n[i-j+1]\theta(j-2) + i\theta(1-j) + j-1), \quad (\text{S12})$$

where  $\theta(x)$  denotes the Heaviside step function. One can henceforth prove by induction that the  $n$ -th order correction

$c_n = s_n - s_{n-1}$  is given by

$$c_n = \frac{[h^{(0)}]^n}{[h^{(1)}]^{2n-1}} \frac{\det \mathcal{A}_n}{(n-1)!} \quad (\text{S13})$$

with the symbolic convention  $\det \mathcal{A}_1 \equiv 1$ . Therefore,  $-\lambda_0$ , the exact root of  $h(s)$ , which is closest to the origin, is given by  $s_r = \sum_{k=1}^{\infty} c_k$ . This completes the proof of Eq. (2) in the main text  $\square$

b) The FPT long-time asymptotics are obtained using Cauchy's theorem

$$\varphi(t) \sim \lim_{s \rightarrow -\lambda_0} [(s + \lambda_0) \tilde{\varphi}(s) e^{st}], \quad (\text{S14})$$

where the contour used to evaluate the residue is chosen to enclose  $-\lambda_0$  such that  $\Re(s) < \lambda_0$ . To do so, we need to find the leading order term of a (formal) partial fraction expansion of  $\tilde{\varphi}(s)$ . We rewrite the moment expansion in Eq. (S1) as a limit of  $n$ th order Taylor polynomial  $\mathcal{P}_n(s)$  with  $n \rightarrow \infty$

$$\tilde{\varphi}(s) = \lim_{n \rightarrow \infty} \left( \sum_{k=0}^n \frac{(-s)^k}{k!} \langle T^k \rangle + \mathcal{R}_{n+1} \right), \quad (\text{S15})$$

with Taylor's remainder theorem assuring the convergence of  $\lim_{n \rightarrow \infty} \mathcal{R}_{n+1} = 0$ . Next we use the relation inverse to the one leading from Eq. (S1) to Eq. (S2) to obtain after some rearrangements

$$\tilde{\varphi}(s) = \lim_{n \rightarrow \infty} \frac{\sum_{k=0}^n g^{(k)}(x_0) s^k / k!}{\sum_{k=0}^n h^{(k)}(x_a) s^k / k!} = \lim_{n \rightarrow \infty} \left( \frac{g^{(n)}}{h^{(n)}} + \frac{\sum_{k=0}^{n-1} \left[ g^{(k)} - \frac{g^{(n)}}{h^{(n)}} h^{(k)} \right] s^k / k!}{\sum_{k=0}^n h^{(k)} s^k / k!} \right), \quad (\text{S16})$$

where we omitted the explicit dependence on  $x_a$  and  $x_0$  and formally carried out a long division in the second step, using the fact that all  $g^{(n)}/n!$ ,  $h^{(n)}/n!$  are finite and well behaved. As by the assumptions of S1 the first term on the right of Eq. (S16) converges as  $n \rightarrow \infty$ , and so does the left side of Eq. (S16), then by necessity the second term on the right of Eq. (S16) converges as well. To isolate the first term of the partial fraction expansion of the second term in Eq. (S16) we carry out a second long division. Introducing the shorthand notation  $b_k = h^{(k)}(x_a)/k!$  leads to

$$\sum_{k=0}^n b_k s^k = (s + \lambda_0) \sum_{k=1}^n c_{n-k} s^k + \sum_{k=0}^n b_k (-\lambda_0)^k, \quad (\text{S17})$$

where  $c_{n-k} \equiv \sum_{l=1}^k b_{n-k+l} (-\lambda_0)^{l-1}$ ,  $\lim_{n \rightarrow \infty} \sum_{k=0}^n b_k (-\lambda_0)^k = 0$  and we omitted the details of the calculation as they are tedious but straightforward. As a result we can write

$$\tilde{\varphi}(s) = \lim_{n \rightarrow \infty} \left( \frac{g^{(n)}}{h^{(n)}} + \frac{\sum_{k=0}^{n-1} \left[ g^{(k)} - \frac{g^{(n)}}{h^{(n)}} h^{(k)} \right] s^k / k!}{(s + \lambda_0) \sum_{k=1}^n c_{n-k} s^{n-k}} \left[ 1 + \frac{\sum_{k=0}^n b_k (-\lambda_0)^k}{(s + \lambda_0) \sum_{k=1}^n c_{n-k} s^{n-k}} \right]^{-1} \right), \quad (\text{S18})$$

where for now we still have  $s \neq -\lambda_0$  (the limit  $s \rightarrow -\lambda_0$  in Eq. (S14) is taken at the end). Noticing that  $\sum_{k=1}^n c_{n-k} s^{n-k} \neq 0$  for any large  $n$  (since  $-\lambda_0$  is a simple pole of  $\tilde{\varphi}(s)$ ; see also previous section) as well as the fact that for any large  $n$  we have  $\sum_{k=0}^n b_k (-\lambda_0)^k \ll 1$  (in fact one can check by explicit computation that  $|\sum_{k=0}^n b_k (-\lambda_0)^k|$  with  $\lambda_0$  in Eq. (2) in the main text, uniformly converges to 0 with increasing  $n$ ) we can Taylor expand the term

$$\left[ 1 + \frac{\sum_{k=0}^n b_k (-\lambda_0)^k}{(s + \lambda_0) \sum_{k=1}^n c_{n-k} s^{n-k}} \right]^{-1} = \sum_{l=0}^{\infty} \left( -\frac{\sum_{k=0}^n b_k (-\lambda_0)^k}{(s + \lambda_0) \sum_{k=1}^n c_{n-k} s^{n-k}} \right)^l \equiv \mathcal{T}_n \quad (\text{S19})$$

and  $\lim_{n \rightarrow \infty} \mathcal{T}_n = 1$ . Moreover, it is easy to show that

$$\frac{\sum_{k=0}^{n-1} \left[ g^{(k)} - \frac{g^{(n)}}{h^{(n)}} h^{(k)} \right] s^k / k!}{(s + \lambda_0) \sum_{k=1}^n c_{n-k} s^k} = \frac{F(s)}{s + \lambda_0} + \frac{G_{n-2}(s)}{\sum_{p=0}^{n-1} c_p s^p} \quad (\text{S20})$$

with  $G_{n-2}(s)$  being some  $n-2$  degree polynomial in  $s$  and

$$F(s) = \frac{\sum_{k=0}^{n-1} \left[ g^{(k)} - \frac{g^{(n)}}{h^{(n)}} h^{(k)} \right] s^k / k!}{\sum_{k=0}^{n-1} \sum_{l=1}^{n-k} b_{k+l} (-\lambda_0)^{k+l-1}}. \quad (\text{S21})$$

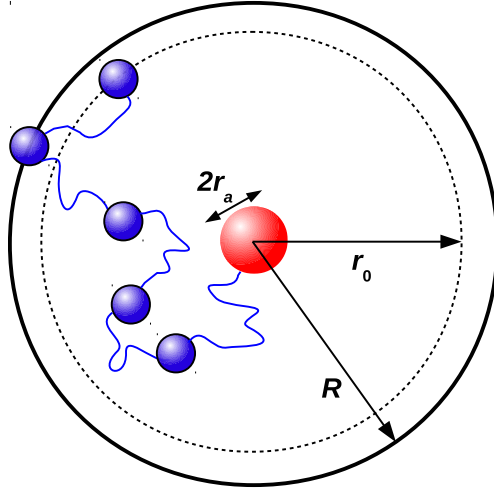

FIG. S1: Schematic of the FPT problem in hyperspherically symmetric media with a reflecting confining boundary at  $R$  and a centered perfectly absorbing target with a radius  $r_a$  (red sphere).

Using this in Eq. (S18) we obtain

$$\lim_{n \rightarrow \infty} \left( \frac{g^{(n)}}{h^{(n)}} + \frac{F(s)\mathcal{T}_n}{s + \lambda_0} + \frac{G_{n-2}(s)\mathcal{T}_n}{\sum_{p=0}^{n-1} c_p s^p} \right). \quad (\text{S22})$$

Since  $\mathcal{T}_n$  converges absolutely to 1 as  $n \rightarrow \infty$  (as by definition  $-\lambda_0$  is a root of  $\sum_{k=0}^n b_k s^k$ ), then by Mertens' theorem [2] we find that

$$\lim_{n \rightarrow \infty} \frac{F(s)\mathcal{T}_n}{s + \lambda_0} = \frac{\lim_{n \rightarrow \infty} F(s)}{s + \lambda_0} \quad \text{and} \quad \lim_{n \rightarrow \infty} \frac{G_{n-2}(s)\mathcal{T}_n}{\sum_{p=0}^{n-1} c_p s^p} = \lim_{n \rightarrow \infty} \frac{G_{n-2}(s)}{\sum_{p=0}^{n-1} c_p s^p} < \infty. \quad (\text{S23})$$

As we also have  $\lim_{n \rightarrow \infty} \frac{g^{(n)}}{h^{(n)}} < \infty$  we can now compute the limit in Eq. (S14) by using Eq. (S23) in Eq. (S22) to obtain the final result in Eq. (6) in the main text  $\square$

The above approach should in fact hold for all FPT densities decaying exponentially for long times as it rests only on one additional assumption, namely that  $\lim_{n \rightarrow \infty} \frac{g^{(n)}}{h^{(n)}} < \infty$ , which appears to be a necessary consequence of the positivity and finiteness of moments of a probability density with strictly positive support. The proof of this conjecture is, however, beyond the scope of the present work.

### ANALYTICAL SOLUTIONS FOR $\tilde{\varphi}(s)$ FOR SPECIFIC CASES

In the analysis of FPT statistics of diffusion in fractal media and diffusion under the influence of a radial bias we consider hyperspherically symmetric systems as depicted in Fig. S1.

#### S3. Mean field model of diffusion in fractal media

The FPT problem for diffusion in fractal media is described on the mean field level with the operator  $\hat{L}_{d_f}^{d_w} = D_{d_w} r^{1-d_f} \partial_r (r^{1+d_f-d_w} \partial_r)$  [4] under zero-flux boundary conditions at  $r = R$  and perfectly absorbing boundary conditions at  $r = r_a$ . The exact Laplace transform of the FPT density starting from a dimensionless radius  $x_0$  for diffusion in fractal media (see main text for definition of the dimensionless units) can be shown to be given by

$$\tilde{\varphi}(s) = \left( \frac{x_0}{x_a} \right)^\nu \frac{\mathcal{D}_{\nu,-}(\hat{x}_0 \sqrt{s}, \sqrt{s})}{\mathcal{D}_{\nu,-}(\hat{x}_a \sqrt{s}, \sqrt{s})} \quad (\text{S24})$$

with  $-\frac{1}{2} \leq \nu = \frac{3}{2} - \frac{d_f+1}{d_w} < \frac{3}{2}$ , and where we introduced the auxiliary function

$$\mathcal{D}_{\nu,\pm}(x, y) = I_\nu(x)K_{\nu\pm 1}(y) + K_\nu(x)I_{\nu\pm 1}(y), \quad (\text{S25})$$

and where  $I_\nu(x)$  and  $K_\nu(x)$  denote the modified Bessel function of the first and second kind, respectively. Using the series expansions for  $I_\nu(x)$  and  $K_\nu(x)$  in [5] one can show that the coefficients  $h^{(n)}, g^{(n)}$  (note that these only differ in the positional variable  $x_0$  versus  $x_a$ ) for  $\nu \neq 0$  are given as

$$g^{(n)} = \frac{n!\pi}{4^n \sin(\pi\nu)} \left( \sum_{l=0}^n \frac{x_0^{2l}}{l!(n-l)!\Gamma(l+1-\nu)\Gamma(n-l+\nu)} - \sum_{l=0}^{n-1} \frac{\theta(n-1)x_0^{2(l+\nu)}}{l!(n-1-l)!\Gamma(l+1+\nu)\Gamma(n-l+1-\nu)} \right), \quad (\text{S26})$$

or, written more compactly using the Gauss hypergeometric functions [5],

$$g^{(n)} = \frac{n!\pi}{4^n \sin(\pi\nu)} \left( \frac{{}_2F_1(-n, 1-n-\nu, 1-\nu; x_0^2)}{\Gamma(1+n)\Gamma(1-\nu)\Gamma(n+\nu)} - \theta(n-1) \frac{x_0^{2\nu} {}_2F_1(1-n, \nu-n, 1+\nu; x_0^2)}{\Gamma(n)\Gamma(1-\nu+n)\Gamma(1+\nu)} \right). \quad (\text{S27})$$

$h^{(n)}$  is obtained from  $g^{(n)}$  by making the substitution  $x_0 \rightarrow x_a$ . In the particular case of  $\nu = \frac{1}{2}$  this simplifies to  $g^{(n)} = \frac{n!(1-x_0)^{2n}}{(2n)!}$  and for  $\nu = -\frac{1}{2}$  we have  $g^{(n)} = \frac{n!(1-x_0)^{2n}(\frac{2n}{x_0}+1)}{(2n+1)!}$ . Using the asymptotic formulas of  ${}_2F_1(a, b, c; z)$  for  $|a|, |b| \rightarrow \infty$  in [5] one can show that  $\lim_{n \rightarrow \infty} \frac{g^{(n)}}{h^{(n)}} = 0$ , as required in section S2. For the sake of completeness we also give the result for the special case  $\nu = 0$ :

$$g^{(n)} = \frac{x_0^{2n}}{4^n n!} + \sum_{l=0}^{n-1} \frac{n!x_0^{2(n-l-1)}}{4^{n-1}l!(n-l-1)!^2(l+1)!} \left( -\log(x_0) - \gamma - \frac{\psi(l+1) + \psi(l+2)}{2} + \frac{(n-l-1)!^2}{(n-l)!^2} [\psi(n-l+1) + \gamma] \right), \quad (\text{S28})$$

where  $\psi(1) = -\gamma$  and  $\psi(k \geq 2) = \sum_{i=1}^{k-1} k^{-1}$  and  $\gamma \simeq 0.5772$  denotes the Euler-Mascheroni constant [5].

The short-time asymptotic is derived using asymptotic formulas for the modified Bessel functions in [5]. We find  $\lim_{x,y \rightarrow \infty} \mathcal{D}_{\nu,\pm}(x, y) \sim \frac{\cosh(y-x)}{\sqrt{xy}}$ , in turn leading to

$$\tilde{\wp}(s) \sim \left( \frac{x_0}{x_a} \right)^{\nu-1/2} e^{-\sqrt{s}(\hat{x}_0 - \hat{x}_a)} \xrightarrow{\mathcal{L}^{-1}} \wp(t) \sim \left( \frac{x_0}{x_a} \right)^{\nu-1/2} \frac{\hat{x}_0 - \hat{x}_a}{2\sqrt{\pi t^3}} e^{-(\hat{x}_0 - \hat{x}_a)^2/4t}, \quad (\text{S29})$$

valid for  $t \lesssim \hat{x}_0^2, \hat{x}_a^2$ .

On the intermediate time-scale we have  $1 \ll \sqrt{s} \ll \hat{x}_a^{-1}, \hat{x}_0^{-1}$  such that  $K_\nu(\sqrt{s}) \rightarrow 0$  and we end up with  $\tilde{\wp}(s) \sim \left( \frac{x_0}{x_a} \right)^\nu \frac{K_\nu(\sqrt{s}\hat{x}_0)}{K_\nu(\sqrt{s}\hat{x}_a)}$ . With the power series expansions of  $K_\nu(z)$  for small  $z$  we find after some algebraic manipulations

$$\tilde{\wp}(s) \sim \left( \frac{x_0}{x_a} \right)^{2\nu\theta(\nu)} \frac{1 - \frac{\Gamma(1-|\nu|)}{\Gamma(1+|\nu|)} \left[ \frac{\sqrt{s}\hat{x}_0}{2} \right]^{2|\nu|}}{1 - \frac{\Gamma(1-|\nu|)}{\Gamma(1+|\nu|)} \left[ \frac{\sqrt{s}\hat{x}_a}{2} \right]^{2|\nu|}} \quad (\text{S30})$$

valid for  $[\Gamma(1+|\nu|)/\Gamma(2-|\nu|)]^{1/(1-|\nu|)}(\hat{x}_0/2)^2 \ll t \ll 1$ . Expanding the denominator and truncating the resulting series after the first correction to the leading order behavior we have

$$\tilde{\wp}(s) \sim \left( \frac{x_0}{x_a} \right)^{2\nu\theta(\nu)} \left( 1 - \frac{\Gamma(1-|\nu|)}{\Gamma(1+|\nu|)} \left[ \left( \frac{\hat{x}_0}{2} \right)^{2|\nu|} - \left( \frac{\hat{x}_a}{2} \right)^{2|\nu|} \right] s^{|\nu|} - \left[ \frac{\Gamma(1-|\nu|)}{\Gamma(1+|\nu|)} \right]^2 \left[ \left( \frac{\hat{x}_0\hat{x}_a}{4} \right)^{2|\nu|} - \left( \frac{\hat{x}_a}{2} \right)^{4|\nu|} \right] s^{2|\nu|} \right). \quad (\text{S31})$$

Eq. (S31) is slowly varying and can be inverted with Feller's version of a Tauberian theorem (Example c, pp. 447 in [1]) to give the result presented in Eq. (10) in the main text. Using the Tauberian theorem for the special case  $\nu = 0$  we in turn obtain  $\wp(t) \sim 2 \log(\frac{x_0}{x_a})/[t(\log(t) - 2 \log(x_a))^2]$ .

Moreover, it follows from Eq. (S26) that the first order correction term in Eq. (4) in the main text in the limit  $x_a \rightarrow 0$  becomes for  $\nu < 0$

$$\lim_{x_a \rightarrow 0} \frac{h^{(2)}(x_a)}{h^{(1)}(x_a)^2} \sim \hat{x}_a^{-2\nu} \frac{-\nu(1-\nu)}{2-\nu} \quad (\text{S32})$$

and

$$\lim_{x_a \rightarrow 0} \frac{h^{(2)}(x_a)}{h^{(1)}(x_a)^2} \sim \frac{1}{2 \log(\hat{x}_a)^2} \quad (\text{S33})$$

for  $\nu = 0$ . The vanishing of the correction terms gives rise to Poisson-like long-time asymptotics in Eqs. (11) and (12).

#### S4. Taylor dispersion

Taylor dispersion is described by the advection-diffusion operator  $\hat{L}_T = -v\partial_r + D\partial_r^2$  with absorbing boundary conditions at  $r = 0$  and reflecting boundary conditions at  $r = R$ . Here the exact Laplace transform of the FPT density to the origin if starting from  $x_0$  for diffusion in a linear potential reads

$$\tilde{\varphi}(s) = e^{-\text{Pe}x_0} \frac{\sqrt{\text{Pe}^2 + s} \cosh \left[ \sqrt{\text{Pe}^2 + s}(1 - x_0) \right] - \text{Pe} \sinh \left[ \sqrt{\text{Pe}^2 + s}(1 - x_0) \right]}{\sqrt{\text{Pe}^2 + s} \cosh \left[ \sqrt{\text{Pe}^2 + s} \right] - \text{Pe} \sinh \left[ \sqrt{\text{Pe}^2 + s} \right]}, \quad (\text{S34})$$

where  $\text{Pe}$  is defined in the main text. Using a power series expansion for the hyperbolic functions as well as the binomial theorem  $(1+x)^k = \sum_{i=0}^k \binom{k}{i} x^i$  we find upon some manipulations and using the series expansion for the modified Bessel function of the first kind  $I_\nu(y)$  the exact result

$$g^{(n)}(z) = \sqrt{\pi} e^{\text{Pe}z} \text{Pe}^{-2n} \left( \frac{z}{2} \right)^{n+1/2} [I_{n-1/2}(z) - \text{sgn}(\text{Pe}) I_{n+1/2}(z)] \quad (\text{S35})$$

with  $z = (1-x)$  and  $h^{(n)} = g^{(n)}(1)$ . Using the asymptotic formulas for  $I_{\nu \rightarrow \infty}(z)$  in [5] one can show that  $\lim_{n \rightarrow \infty} \frac{g^{(n)}}{h^{(n)}} = 0$ , as required in section S2.

The short- and intermediate-time scale behavior is derived from Eq. (S34) by taking the limit  $(\text{Pe}^2 + s) \rightarrow \infty$  and using the first shifting theorem for Laplace transforms

$$\tilde{\varphi}(s) \sim e^{-\text{Pe}x_0} e^{-\sqrt{\text{Pe}^2 + s}x_0}, \quad \xrightarrow{\mathcal{L}^{-1}} \quad \varphi(t) \sim \Phi(t; x_0) e^{-\text{Pe}x_0 - \text{Pe}^2 t} \quad (\text{S36})$$

thereby leading directly to Eq. (13) in the main text.

In the limit  $\text{Pe} \rightarrow \infty$  (strong bias away from the target) we find using Eq. (S35) that the first correction term to  $\lambda_0$  in Eq. (4) in the main text vanishes exponentially,

$$\lim_{\text{Pe} \rightarrow \infty} \frac{h^{(2)}}{h^{(1)2}} \sim 4e^{-2\text{Pe}} \text{Pe}, \quad (\text{S37})$$

thus giving rise to Poisson-like long-time asymptotics.

#### S5. Radially biased diffusion in 2d

Radially biased 2D diffusion is described by the operator  $\hat{L}_{2D} = D\partial_r^2 + (D - v_0)r^{-1}\partial_r$  [6]. The exact Laplace transform of the FPT density starting from a dimensionless radius  $x_0$  to a centered target with radius  $x_a$  for 2d diffusion under the influence of a radial bias is given by [6]

$$\tilde{\varphi}(s) = \left( \frac{x_0}{x_a} \right)^{-\mu} \frac{\mathcal{D}_{\mu,+}(x_0\sqrt{s}, \sqrt{s})}{\mathcal{D}_{\mu,+}(x_a\sqrt{s}, \sqrt{s})} \quad (\text{S38})$$

with  $\mu = \text{Pe}/2$  and  $\mathcal{D}_{\mu,+}$  defined in Eq. (S25). Using the series expansion of the respective modified Bessel functions [5] the coefficients entering Eqs. (1) to (6) in the main text read

$$g^{(n)} = \frac{-n!\pi x^\mu}{4^n \sin(\pi\mu)} \left( \sum_{l=0}^n \frac{x_0^{2(n-l)}}{l!(n-l)!\Gamma(l-\mu)\Gamma(n-l+1+\mu)} - \sum_{l=0}^{n-1} \frac{\theta(n-1)x_0^{2(n-1-l-\mu)}}{l!(n-1-l)!\Gamma(l+2+\mu)\Gamma(n-l-\mu)} \right) \quad (\text{S39})$$

and  $h^{(n)}$  is obtained as before by the substitution  $x_0 \rightarrow x_a$ . Eq. (S39) can be written more compactly using the Gauss hypergeometric functions [5]:

$$g^{(n)} = \frac{-n! \pi x^\mu x_0^{2n}}{4^n \sin(\pi \mu)} \left( \frac{{}_2F_1(-n, -n + \mu, -\mu; x_0^{-2})}{\Gamma(1+n)\Gamma(1+n-\mu)\Gamma(-\mu)} - \theta(n-1) \frac{x_0^{-2(1+\nu)} {}_2F_1(1-n, 1-n+\mu, 2-\mu; x_0^{-2})}{\Gamma(n)\Gamma(2-\mu)\Gamma(n-\mu)} \right). \quad (\text{S40})$$

Using the asymptotic formulas of  ${}_2F_1(a, b, c; z)$  for  $|a|, |b| \rightarrow \infty$  in [5] one can show that  $\lim_{n \rightarrow \infty} \frac{g^{(n)}}{h^{(n)}} = 0$ , as required in section S2.

It can be shown that the short- and intermediate-time asymptotics are equivalent to those found in Eqs. (S29) and (S30) but with the substitution  $\nu = -\mu$ . Similarly, the correction term in Eq. (4) in the main text in the limit  $\text{Pe} \rightarrow \infty$  (strong outward bias) vanishes

$$\lim_{x_a \rightarrow 0} \frac{h^{(2)}(x_a)}{h^{(1)}(x_a)^2} \sim \frac{\text{Pe}}{2} x_a^{\text{Pe}}, \quad (\text{S41})$$

giving rise to Poisson-like long-time asymptotics.

### S6. Ornstein-Uhlenbeck process

The overdamped escape from a harmonic potential involves the Ornstein-Uhlenbeck operator  $\hat{L}_{OU} = (m\kappa)^{-1}(\partial_r U(r) + k_B T \partial_r^2)$  [7] with absorbing BCs at  $a$  and natural BCs at  $-\infty$ . The exact Laplace transform of the FPT density starting from a dimensionless  $x_0$  over a barrier at  $x_a$  ( $x_a > x_0$ ) for an overdamped particle in harmonic confinement is given by [7]

$$\tilde{\varphi}(s) = e^{(x_0^2 - x_a^2)/4} \frac{D_{-s}(-x_0)}{D_{-s}(-x_a)} \equiv \frac{H_{-s}(-x_0/\sqrt{2})}{H_{-s}(-x_a/\sqrt{2})}, \quad (\text{S42})$$

in terms of Weber and generalized Hermite functions, respectively [5]. For the OU process the coefficients  $h^{(k)}, g^{(k)}$  are given in terms of  $H_0^{n,0}(x) \equiv (-1)^n \frac{\partial^n}{\partial \alpha^n} H_\alpha(-\frac{x}{\sqrt{2}})|_{\alpha=0}$ , which are readily implemented in the Mathematica software.

One can confirm numerically that  $\frac{g^{(n)}}{h^{(n)}}$  converges rapidly to 0 with increasing  $n$ . While it is possible to prove this analytically as well, this task will be reserved for a separate longer publication.

The short- and intermediate-time scale asymptotics are obtained from the expansion of  $D_{-s}(-x_0)$  for  $s \gg x_{0,a}^2$  [5] leading to

$$\tilde{\varphi}(s) \sim e^{(x_0^2 - x_a^2)/4} e^{-\sqrt{s}(x_a - x_0)} \frac{1 + \frac{|x_0|^3}{24}s - \frac{x_0^2}{16}s^2}{1 + \frac{x_a^3}{24}s - \frac{x_a^2}{16}s^2}. \quad (\text{S43})$$

The inversion of both factors in Eq. (S43) leads to the convolution Eq. (15) in the main text.

As for the long-time limit it is in fact sufficient to inspect the term  $\frac{h^{(2)}(x_a)}{h^{(1)}(x_a)^2}$ . Using the exact result for  $H_0^{1,0}$  in the main text one can show [5] that we have (note that the argument in  $H_0^{n,0}$  is actually negative)

$$\lim_{|x| \rightarrow \infty} H_0^{1,0}(x) \sim \sqrt{2\pi} e^{x^2/2} (|x|^{-1} - x^{-1}) + \log(|x|). \quad (\text{S44})$$

Moreover, using the formulas in [5] we also have that

$$\lim_{|z| \rightarrow \infty} H_{-s}(z) \sim -\sqrt{\pi} \frac{e^{z^2} z^{-s}}{z\Gamma(s)} e^{i\pi s} \quad \text{Arg}(z) \geq \frac{\pi}{2} \quad (\text{S45})$$

(note that in our case  $z$  is real and negative) to obtain after taking the second derivative

$$\lim_{|x| \rightarrow \infty} H_0^{2,0}(x) \sim 2\sqrt{2\pi} \frac{\gamma e^{x^2/2}}{x}, \quad (\text{S46})$$

such that

$$\lim_{x_a \rightarrow \infty} \frac{h^{(2)}(x_a)}{h^{(1)}(x_a)^2} \sim 16x\gamma e^{-x_a^2/2} \sqrt{2/\pi}, \quad (\text{S47})$$

giving rise to Poisson-like long-time asymptotics in the high barrier limit. Conversely, in the limit  $x_a \ll -1$  ( $x_0 < x_a$ ) we obtain using  $\lim_{z \rightarrow \infty} D_{-s}(z) \sim e^{-z^2/4} x^{-s}$  [5] and taking  $x^{-s} = e^{-s \log(x)}$  the deterministic limit

$$\tilde{\wp}(s) \sim e^{-s \log(x_0/x_a)} \xrightarrow{\mathcal{L}^{-1}} \wp(t) \sim \delta(t - \log[x_0/x_a]). \quad (\text{S48})$$

Equivalently we recover  $\langle T(x_0) \rangle \sim \log(x_0/x_a)$ .

- 
- [1] Feller W, *An Introduction to Probability Theory and Its Applications vol. II.* (Wiley, New York 1968).
  - [2] Whittaker ET, *A Course of Modern Analysis: An Introduction to the General Theory of Infinite Series and of Analytic Functions, with an Account of the Principal Transcendental Functions.*, Cambridge University Press, Cambridge (1902).
  - [3] Householder AS, *The numerical treatment of a single nonlinear equation* (McGraw-Hill, New York 1970).
  - [4] B. O'Shaughnessy and I. Procaccia, *Analytical solutions for diffusion on fractal objects.* .Phys. Rev. Lett. 54, 455 (1985).
  - [5] Abramowitz, M. and Stegun, I. A. *Handbook of mathematical functions.* Dover, New York, (1970).
  - [6] Koplik J, Redner S, and Hinch E J, *Universal and nonuniversal first-passage properties of planar multipole flows.* Phys. Rev. Lett. 74, 82 (1995).
  - [7] Siegert A J F, *On the First Passage Time Probability Problem.* Phys. Rev. 81, 617 (1951).
